# Supplementary material for: Qwen2.5 Technical Report
Source: arXiv:2412.15115 source file (2025-01-03)
Supplement: Supplementary file 1 [file appendix.tex]

% 下面的coding和多语言的细节，考虑放到附录。上面的总表其实也已经有所体现
\section{Appendix}
\label{sec:appendix}

\subsection{More Evaluation Results}

Here we present more detailed evaluation results of our Qwen2 models and the baselines. Specifically, we demonstrate the coding performance in different code languages, and the language understanding performance in multilingual evaluation.

\subsubsection{Coding}

Instead of simply evaluating the models on the conventional coding benchmarks, namely HumanEval and MBPP, we extend the evaluation for coding to comprehensively test the models' capabilities in coding problem-solving. Specifically, we follow the practice of CodeQwen~\citep{codeqwen} and implement the evaluation of EvalPlus~\citep{evalplus} and Multipl-E~\citep{multiple}. Specifically, EvalPlus includes HumanEval and MBPP, as well as their new versions with extended test cases. MultiPL-E includes test sets in different code languages, including Python, C++, Java, PHP, TypeScript, C\#, Bash, JavaScript and Go, and it aims at testing the capability of LLMs in understanding and generating codes in different languages.

% \begin{table}[t]
% \centering
% \small
% \caption{Performance of 70B.}
% \label{tab:to_sota}
% \begin{tabular}{l|ccccc}
% \toprule
% \textbf{Datasets} &\textbf{Mixtral-8x22B}  & \textbf{DeepSeek V2} & \textbf{Llama-3-70B} & \textbf{Qwen1.5-110B} &\textbf{Qwen2-72B} \\
% \midrule
% \multicolumn{6}{c}{\textit{EvalPlus (Python)}} \\
% \midrule
% HumanEval & 46.3 & 45.7 & 48.2 & 46.3 & \textbf{64.6} \\
% HumanEval+ & 40.2 & 40.9 & 42.1 & 43.3 & \textbf{56.1} \\
% MBPP       & 71.7 & 73.9 & 70.4 & 66.9 & \textbf{76.9} \\
% MBPP+     & 58.1 & 59.6 & 58.4 & 55.1 & \textbf{63.9} \\
% \midrule
% Avg. & 54.1 & - & 54.8 & 52.9 & \textbf{65.4} \\
% \midrule
% \multicolumn{6}{c}{\textit{MultiPL-E}} \\
% \midrule
% Python      & 46.3 &  ?  & 45.7 & 45.1 & \textbf{64.0} \\
% C++         & 54.0 &  ?  & 49.6 & 43.5 & \textbf{67.7} \\
% Java        & 46.2 &  ?  & 41.1 & 47.5 & \textbf{50.0} \\
% PHP         & 37.2 &  ?  & 45.9 &  42.8 & \textbf{60.2} \\
% TypeScript  & 54.0 &  ?  & 55.9 &  47.2 &  \textbf{64.8} \\
% C\#          & 52.5 &  ?  & 54.4 & 44.3 &  \textbf{62.7} \\
% Bash        & 28.4 &  ?  & 25.9 & 17.7 &  \textbf{44.3} \\
% JavaScript  & 54.6 &  ?  & 51.5 &  46.6 &  \textbf{62.7} \\
% Go          & 35.1 &  ?  & 31.8 & 27.9 & \textbf{38.3} \\
% \midrule
% Avg.        & 45.4 &  ?  & 44.6  & 40.3 & \textbf{57.2} \\
% \bottomrule
% \end{tabular}
% \end{table}

\begin{table}[t]
\centering
\caption{Performance of 70B.}
\label{tab:code-70}
\setlength{\tabcolsep}{5pt}
\begin{tabular}{@{}l|ccccc@{}}
\toprule
\textbf{Datasets} &\textbf{Mixtral-8x22B}   & \textbf{Llama-3-70B} & \textbf{Qwen1.5-72B} & \textbf{Qwen1.5-110B} &\textbf{Qwen2-72B} \\
\midrule
\multicolumn{6}{c}{\textit{EvalPlus (Python)}} \\
\midrule
HumanEval & 46.3  & 48.2  & 46.3 & 54.3 & \textbf{64.6} \\
HumanEval+ & 40.2  & 42.1 & 43.3 & 46.3 & \textbf{56.1} \\
MBPP       & 71.7  & 70.4 & 66.9 & 70.9 & \textbf{76.9} \\
MBPP+     & 58.1  & 58.4 & 55.1 & 59.4 & \textbf{63.9} \\
\midrule
Avg. & 54.1 & 54.8 & 52.9 & 57.7 & \textbf{65.4} \\
\midrule
\multicolumn{6}{c}{\textit{MultiPL-E}} \\
\midrule
Python      & 46.3  & 45.7 & 45.1 & 55.5 & \textbf{64.0} \\
C++         & 54.0  & 49.6 & 43.5 & 52.8 & \textbf{67.7} \\
Java        & 46.2  & 41.1 & 47.5 & 51.9 & \textbf{50.0} \\
PHP         & 37.2  & 45.9 &  42.8 & 52.2 &\textbf{60.2} \\
TypeScript  & 54.0  & 55.9 &  47.2 & 57.2  & \textbf{64.8} \\
C\#          & 52.5  & 54.4 & 44.3 & 56.9  & \textbf{62.7} \\
Bash        & 28.4 & 25.9 & 17.7 & 37.3 & \textbf{44.3} \\
JavaScript  & 54.6 & 51.5 &  46.6 & 57.8 &  \textbf{62.7} \\
Go          & 35.1  & 31.8 & 27.9 & 38.3 & \textbf{38.3} \\
\midrule
Avg.        & 45.4  & 44.6  & 40.3 & 51.0 & \textbf{57.2} \\
\bottomrule
\end{tabular}
\end{table}

\begin{table}[t]
\centering
\caption{Performance of 57B-A14B.}
\label{tab:code-57a14}
\begin{tabular}{@{}l|cccc@{}}
\toprule
\textbf{Datasets} &\textbf{Mixtral-8x7B}   & \textbf{Yi-1.5-34B} & \textbf{Qwen1.5-32B}  &\textbf{Qwen2-MoE-57B-A14B} \\
\midrule
\multicolumn{5}{c}{\textit{EvalPlus (Python)}} \\
\midrule
HumanEval & 37.2  & 46.3  & 43.3 & \textbf{53.0} \\
HumanEval+ & 31.1  & 40.2 & 40.2  & \textbf{46.3} \\
MBPP       & 63.9  & 65.5 & 64.2 & \textbf{71.9} \\
MBPP+     & 53.6  & 55.4 & 53.9 & \textbf{57.4} \\
\midrule
Avg. & 46.4 & 51.9 & 50.4 & \textbf{57.2} \\
\midrule
\multicolumn{5}{c}{\textit{MultiPL-E}} \\
\midrule
Python      & 37.2 & 36.6 & 43.3 & \textbf{53.7} \\
C++         & 41.8  & \textbf{48.4} & 41.6 & \textbf{48.4} \\
Java        & 39.8  & 48.1  & 35.4 & \textbf{52.5} \\
PHP         & 38.5 &  35.4 & 35.4 &\textbf{53.4} \\
TypeScript   & 47.1 &  44.7 & 46.5  & \textbf{59.1} \\
C\#          & 48.1  & 50.6 & 48.1  & \textbf{53.2} \\
Bash        & 13.9 & 12.0 & 13.3  & \textbf{29.7} \\
JavaScript  & 45.3  & 39.8 & 44.7 &  \textbf{48.4} \\
Go          & 20.7  & 26.6  & 26.6 & \textbf{29.9} \\
\midrule
Avg.        & 41.6  & 37.9 & 41.8 & \textbf{47.6} \\
\bottomrule
\end{tabular}
\end{table}

\begin{table}[t]
\centering
\caption{Performance of 7B.}
\label{tab:code-7}
\begin{tabular}{@{}l|ccccc@{}}
\toprule
\textbf{Datasets} &\textbf{Mixtral-7B}   & \textbf{Gemma-7B} & \textbf{Llama-3-8B}  &\textbf{Qwen1.5-7B} & \textbf{Qwen2-7B} \\
\midrule
\multicolumn{6}{c}{\textit{EvalPlus (Python)}} \\
\midrule
HumanEval & 29.3  & 37.2  & 33.5 & - & \textbf{50.0} \\
HumanEval+ & 24.4  & 28.0 & 29.3 & -  & \textbf{42.7} \\
MBPP       & 51.1  & 50.6 & 53.9 & - & \textbf{59.9} \\
MBPP+     & 40.9  & 42.4 & 44.4 & - & \textbf{47.4} \\
\midrule
Avg. & 36.4 & 39.6 & 40.3 & - & \textbf{50.0} \\
\midrule
\multicolumn{6}{c}{\textit{MultiPL-E}} \\
\midrule
Python      & 29.9 &  35.3 & 29.3 & - & \textbf{50.0} \\
C++         & 31.7  & 34.7 & 27.3 &- & \textbf{40.4} \\
Java        & 31.0  & 23.4  & 25.9 & - & \textbf{37.3} \\
PHP         & 27.3 & 29.2 & 7.5 & - & \textbf{42.2} \\
TypeScript   & 33.9 &  35.2 & 25.2  & - & \textbf{48.4} \\
C\#          & 36.0  & 31.0 & 23.4  & - & \textbf{40.5} \\
Bash        & 9.4 & 8.2 & 8.9  & - & \textbf{23.4} \\
JavaScript  & 36.0  & 40.3 & 32.9 & - & \textbf{47.8} \\
Go          & 22.3  & 23.4  & 16.9 & - & \textbf{29.2} \\
\midrule
Avg.        & 28.6  & 29.0 & 21.9 & - & \textbf{39.9} \\
\bottomrule
\end{tabular}
\end{table}

% \subsection{Multilinguality}
% We curate our multilingual benchmark from different kinds of datasets to thoroughly evaluate Qwen2 series across different languages. These datasets can be grouped into four categories:

% \begin{itemize}
%     \item \textbf{Exam} M3Exam (5-shot, we only choose examples that require no image), IndoMMLU (3-shot)~\citep{koto-etal-2023-indommlu}
% , ruMMLU (5-shot)~\citep{rummlu-mera}, and translated MMLU for the other languages (5-shot).
%     \item \textbf{Understanding} BELEBELE (5-shot)~\citep{belebele}, XCOPA (5-shot)~\citep{xcopa}, XWinograd (5-shot)~\citep{xwinograd}, XStoryCloze (0-shot)~\citep{xstory_cloze} and PAWS-X (5-shot)~\citep{paws-x}
%     \item \textbf{Mathematics} MGSM (8-shot CoT)~\citep{flores}
%     \item \textbf{Translation} Flores-101 (5-shot)~\citep{flores}
% \end{itemize}
